# Supplementary material for: We're Not Gonna Break It! Consistency-Preserving Operators for Efficient Product Line Configuration
Source: arXiv:2204.12918 source file (2022-04-27)
Supplement: Supplementary file 1 [file appendix2_results.tex]

\subsection{Results: Additional Details}
\label{sec:appendix:results}

  \draft{Need a bit of text here to reference the figures etc. Should we have at least some of these figures in the main paper body?}

\begin{draftlist}
Regarding Automotive's results for \SATIBEA:

\item According to the \ACAPULCO\ paper (Section 4 C, attached), the four evolving operations (smart replacement, smart mutation, crossover, and mutation) modify existing solutions without maintaining the best.

\item Checking the source code we can see that \SATIBEA\ removes the worst solutions (even being valid) according to the fitness function, and replaces them with new ones that are generating following the four evolving operations.

\item This is done to promote maximal diversity but for automotive at a specific point (around 1500 evols) \SATIBEA\ is not able to find more valid solutions (currently less than the population size) and starts removing one by one the valid ones (maybe a local optima?) through the "removeWorst" method.

\item I've run it with 1500 evolutions instead of 5000, and at that point (1500 evols) \SATIBEA\ has more valid solutions than in the following evolutions, but in any case valid solutions are less than the whole population. \ACAPULCO\ in contrast fills the whole population with valid solutions.

\item Why this doesn't occurs with other feature models?  Because it is easier to find valid solutions (I've tried \SATIBEA\ for WeaFQAs with 50k instead of 5k evols and it doesn't occurs).

\item Note that Automotive is the only case study that takes much more time in comparison with other case studies (30 seconds vs <3 seconds for the rest of case studies), and this happens for both tools \ACAPULCO\ and \SATIBEA.
\end{draftlist}

\input{plots/wget} 
\input{plots/tankwar}
\input{plots/busybox}
\input{plots/embtoolkit}
\input{plots/linuxdist}
\input{plots/automotive}
